# Supplementary material for: Factors of Influence for Transfer Learning across Diverse Appearance Domains and Task Types
Source: arXiv:2103.13318 source file (2021-11-20)
Supplement: Supplementary file 1 [file A0_appendices_layout.tex]

\input{macros_appendix}

\newcommand{\appendixtitleauthor}[3]{
\bgroup\par\vskip\IEEEtitletopspace\vskip\IEEEtitletopspaceextra
\begin{center}
    \vskip1.0em{}
    {\Huge\sffamily {#1}\par}\relax
  \vskip1.0em\par
  {\lineskip.5em\sffamily\sublargesize {#2}\par
  }
\end{center}
\egroup}

\newcommand{\appendixabstract}[1]{
\bgroup\par\vskip\IEEEtitletopspace\vskip\IEEEtitletopspaceextra
\begin{center}
    %\vskip 1.5em\relax
    \parbox{.922\textwidth}{\footnotesize
        \textbf{Abstract ---} {#1}}%
    \vskip .5em\relax
    \par\noindent\hfill
    \IEEEcompsocdiamondline\hfill\hbox{}\par
    \vskip 1.5em\relax
\end{center}
\egroup}

\thispagestyle{empty}
\setcounter{table}{0}
\setcounter{figure}{0}
\setcounter{equation}{0}
\twocolumn[\begin{@twocolumnfalse}
    \appendixtitleauthor{Supplementary Material}{}{}  
    \appendixabstract{\input{A0_appendices_abstract}}
    \end{@twocolumnfalse}
]

\markboth{Supplementary Material: Factors of Influence}{Supplementary Material: Factors of Influence}
